# Supplementary material for: Randomized Joint Diagonalization of Symmetric Matrices
Source: arXiv:2212.07248 source file (2023-10-23)
Supplement: Supplementary file 1 [file appendix.tex]

\section{Appendix}
\begin{lemma}\label{Perturbation Analysis Old}
Let $A,E \in \reals^{n \times n}$ be symmetric with $\fnorm{E} = \epsilon$. Let $\mathcal{X}_0$  be an eigenspace corresponding to an eigenvalue $\lambda_0$ of $A$. Let $X_0$ be a matrix whose columns are an orthonormal basis of $\mathcal{X}_0$. Denote the distance of $\lambda_0$ to the rest of the spectrum of $A$ by $s_0$, that is, $s_0 = \min\{\abs{\lambda_0 -\nu},\nu: \nu \in \sigma(A), \nu \neq \lambda_0\}$. If $\epsilon  < s_0/2$, then there exists $X_E$ of $A+E$ such that
\begin{enumerate}[label=(\roman*)]
    \item The columns of $X_E$ form a basis of invariant subspace $\mathcal{X}_E$ of $A+E$.
    \item  $(X_E - X_0)^TX_0 = \mathbf{0}$.
    \item $X_E = X_0 + (\lambda_0I - A)\pesudoinverse EX_0 + \Ocal(\epsilon^2)$.
\end{enumerate}
\end{lemma}
\begin{proof}
After an orthogonal similarity transformation we can assume that
\[ A = \begin{bmatrix}
\lambda_0I & 0 \\ 0 & A_{22}
\end{bmatrix}, \mspace{10mu} \det(A_{22} - \lambda_0I) \neq 0, \mspace{10mu} X_0 = \begin{bmatrix}
I \\ 0
\end{bmatrix}, \mspace{10mu} E =  \begin{bmatrix}
E_{11} & E_{12} \\  E_{21} & E_{22}
\end{bmatrix}.\]
By \cite[Theorem 3.6]{MR3205738}, we have
\begin{enumerate}[label=(\roman*')]
    \item The columns of $X_E = \begin{bmatrix} I \\ W_E \end{bmatrix}$ span an invariant subspace of $\mathcal{X}_E$ of $A+E$
    \item The matrix $W_E$ satisfies
    \[\fnorm{W_E - \mathbb{T}^{-1}(E_{21})} \leq  \frac{6}{s_0^2}\epsilon^2 \in \Ocal(\epsilon^2),\]
    where $\mathbb{T} : Z \to Z\lambda_0I - A_{22}Z = (\lambda_0I - A_{22})Z$ is the Sylvester operator.
\end{enumerate}
Obviously, the claim (i) and (ii) follow from (i').

Then $W_E = \mathbb{T}^{-1}(E_{21}) + (W_E -  \mathbb{T}^{-1}(E_{21})) =  \mathbb{T}^{-1}(E_{21}) + \Ocal(\epsilon^2)$. Since $A_{22} - \lambda_0I$ is nonsingular,
\[ \mathbb{T}^{-1}(Z) = (\lambda_0I - A_{22})^{-1}Z .\]
Thus,
\[\begin{split}
    X_E &= X_0 + \begin{bmatrix} \mathbf{0} \\ W_E\end{bmatrix} \\
    &= X_0 + \begin{bmatrix} \mathbf{0} \\ \mathbb{T}^{-1}(E_{21})\end{bmatrix} + \Ocal(\epsilon^2)\\
    &= X_0 + \begin{bmatrix} \mathbf{0} & \mathbf{0}\\ \mathbf{0} & \mathbb{T}^{-1}    \end{bmatrix} \begin{bmatrix} E_{11} \\ E_{21}\end{bmatrix} + \Ocal(\epsilon^2) \\
    &= X_0 + \begin{bmatrix} \mathbf{0} & \mathbf{0}\\ \mathbf{0} & \mathbb{T}^{-1}    \end{bmatrix} EX_0 + \Ocal(\epsilon^2)\\
    &= X_0 + (\lambda_0I - A)\pesudoinverse EX_0 + \Ocal(\epsilon^2),
\end{split}  \]
which is claim (iii).
\end{proof}
With these two lemmas we are in the position to prove the main theorem.
\begin{theorem}
Suppose $\Acal = \{A_k \in \reals^{n \times n}\}_{k=1}^{d}$ is an exactly commuting family. Suppose that there are symmetric matrices $E_k \in \reals^{n \times n}, k \in \{1,\dots,d\}$  such that $\sum_{k=1}^{d}\fnorm{E_k}^2 \leq \epsilon^2$. Let $\tilde{\Acal} = \{\tilde{A_k} = {A_k} + E_k\}$ for $k \in \{1,\dots,d\}$. Let $\Vec{\mu} \sim \mathcal{N}(0, I_d)$ be a standard normal random vector and consider the corresponding linear combination $\tilde{A}(\Vec{\mu}) = \sum_{k=1}^{d} \mu_k\tilde{A_k}$, with $A(\Vec{\mu}), E(\Vec{\mu})$ defined analogously.
 Let $m$ be the number of groups of eigenvalues of $\Acal$ defined as in Section \ref{subsec:exact_correct}. For $\epsilon > 0$, if $\tilde{Q} \in \reals^{n \times n}$ such that $\tilde{Q}^T \tilde{Q} = I_n$ and  $\tilde{Q}^T\tilde{A}(\Vec{\mu})\tilde{Q}$ is diagonal, then for $R>1$,
\[Pr\big((\sum_{k=1}^{d}\fnorm{\offdiag(\tilde{Q}^T\tilde{A}_k\tilde{Q})}^2 \leq R^2 \epsilon^2 + \Ocal(\epsilon^3)\big) \geq 1 - \frac{dm(m-1)}{\sqrt{2\pi}(R-1)}.\]
\end{theorem}
\begin{proof}
Let $\{\Vec{x}_1,...,\Vec{x}_n\}$ be an orthonormal basis consisting of common eigenvectors for $\{A_k\}_{k=1}^d$. Let $\lambda_{ki}$ be the eigenvalue of $x_i$ for the matrix $A_k$ for $i \in [n], k \in \{1,\dots,d\}$. Let $m$ (the number of ``groups" of eigenvalues), $\{n_1,\dots,n_{m+1}\}$, the matrix $\Lambda $ and its columns $\Vec{\Lambda}_i$'s be defined as in Section \ref{subsec:exact_correct}. Then by Theorem \ref{thm:exact}, we know that $A(\mu)$ will share the same $m$ ``groups" of eigenvalues as $A_1,\dots,A_d$, that is, $\lambda_i(\Vec{\mu}) = \lambda_{n_r}(\Vec{\mu}) $ for all $i \in [n_{r},n_{r+1}), r \in \{1,\dots,m\}$,  and for $i,j \in \{1,\dots,m\}$, if $i \neq j$, then $\lambda_{n_i}(\Vec{\mu})  \neq  \lambda_{n_j}(\Vec{\mu})$ with probability $1$. 

Without loss of generality, we may assume $\epsilon$ is sufficiently small.  Consider the random linear combination $\tilde{A}(\Vec{\mu}) = A(\Vec{\mu}) + E(\Vec{\mu})$ . Without loss of generality again,  we consider the first group of eigenvectors. Let matrix $X_1 = \begin{bmatrix} \Vec{x}_1 & \Vec{x}_2 & \dotsb &  \Vec{x}_{n_1-1} \end{bmatrix}$, columns of $X_1$ form an orthonormal basis for the eigensapce $\mathcal{X}_1$ of $\lambda_1(\Vec{\mu})$ for $A(\Vec{\mu})$ with probability $1$. Since $\epsilon$ is sufficiently small, by Lemma \ref{Perturbation Analysis} there exists $\hat{X}_1$ such that:
\begin{enumerate}[label=(\roman*)]
    \item Columns of $\hat{X}_1$ form a basis of an invariant subspace $\tilde{\mathcal{X}}_1$ of $\tilde{A}(\Vec{\mu})$.
    \item For all square matrix $C$ with compatible dimension, because the residual is perpendicular, that is, $(\hat{X_1} - X_1)^TX_1 =\textbf{0} $,  we have $\eunorm{X_1C} \leq \eunorm{\hat{X}_1C}$.
    \item $\hat{X}_1 = X_1 + (\lambda_1(\Vec{\mu})I - A(\Vec{\mu}))\pesudoinverse E(\Vec{\mu})X_1 + \Ocal(\epsilon^2) $. 
\end{enumerate}
   
For any $\tilde{X}_1$ which is an orthonormal basis of $\tilde{\Xcal}_1$, there exist a square matrix $C$ with compatible dimension such that $\tilde{X}_1 = \hat{X}_1 C$. Thus, we have that
\[
    \tilde{X}_1 = Y_1 + (\lambda_1(\Vec{\mu})I - A(\Vec{\mu}))\pesudoinverse E(\Vec{\mu})Y_1 + \Ocal(\epsilon^2),
\]
where $Y_1 = X_1 C$ with $\eunorm{Y_1} \leq \eunorm{\tilde{X}_1} = 1$. Since $\Col(Y_1)$ is at least a subspace of $\mathcal{X}_1$, which corresponds to the first group of eigenvalues, we have $(A_k - \lambda_{k1}I)Y_1 = 0$ for all $k \in \{1,\dots,d\}$.

The above argument works for any $X_i$ which is an orthonormal basis for $\Xcal_i$ for $i \in \{1,\dots,m\}$. Thus, for $i \in \{1,\dots,m\}$, with  $\tilde{\mathcal{X}}_i$ defined as above, for any $\tilde{X}_i$ which is an orthonormal basis of $\tilde{\Xcal}_i$, we have that
\begin{equation}
    \tilde{X}_i = Y_i + (\lambda_{n_i}(\Vec{\mu})I - A(\Vec{\mu}))\pesudoinverse E(\Vec{\mu})Y_i + \Ocal(\epsilon^2),
\end{equation} 
where $\eunorm{Y_i} \leq 1$ and $(A_k - \lambda_{kn_i}I)Y_i =0$ for all $k \in \{1,\dots,d\}$. For the invariant subspaces $\tilde{\Xcal}_i$'s, as $\epsilon$ is sufficiently small, we have that $\tilde{\Xcal}_i \perp \tilde{\Xcal}_j, \forall i \neq j$ and $\bigoplus_{i=1}^{m} \tilde{\Xcal}_i = \reals^n$. In turn, without loss of generality, we can assume $\tilde{Q}= \begin{bmatrix}
\tilde{X}_1 & \dotsb & \tilde{X}_m \end{bmatrix}$. Furthermore, let $Y=\begin{bmatrix}
Y_1 & \dotsb & Y_m \end{bmatrix}$, we have $\eunorm{Y} \leq 1$.

If we view $\tilde{X}_i$ as an orthonormal basis for an approximated eigenspace of $\tilde{A}_k$ with an approxiamted eigenvalue $\lambda_{kn_i}$,  $(\tilde{A}_k - \lambda_{kn_i}I)\tilde{X}_i$ can be thought of as a residual.  Then from (\ref{eq:linearization}), we get for any $k \in \{1,\dots,d\}, i \in \{1,\dots,m\}$, the residual $(\tilde{A}_k - \lambda_{kn_i}I)\tilde{X}_i$ is small  as shown below:
\begin{equation}
    \begin{split}
         (\tilde{A}_k - \lambda_{kn_i}I)\tilde{X}_i &= (A_k - \lambda_{kn_i}I + E_k )(Y_i + (\lambda_{n_i}(\Vec{\mu})I - A(\Vec{\mu}))\pesudoinverse E(\Vec{\mu})Y_i) + \Ocal(\epsilon^2) \\
         &=  (A_k - \lambda_{kn_i}I) (\lambda_{n_i}(\Vec{\mu})I - A(\Vec{\mu}))\pesudoinverse E(\Vec{\mu})Y_i + E_kY_i + \Ocal(\epsilon^2).
    \end{split}
\end{equation}
In turn, small residue can imply small off-diagonal error.
For any $i\in \{1,\dots,m\}$, consider the $i$-th group of columns in $\tilde{Q}^T\tilde{A}_k\tilde{Q}$ for any $k \in \{1,\dots,d\}$,
\[
    \tilde{Q}^T\tilde{A}_k\tilde{X}_i = \tilde{Q}^T(\tilde{A}_k - \lambda_{kn_i}I)\tilde{X}_i + \lambda_{kn_i}\tilde{Q}^T \tilde{X}_i.
\]
Notice that the entries in $\lambda_{kn_i}\tilde{Q}^T \tilde{X}_i$ that corresponds to the off-diagonal entries of $\tilde{Q}^T\tilde{A}_k\tilde{Q}$ are all zero. Thus, we have
\begin{equation}
    \begin{split}
        &\fnorm{\offdiag(\tilde{Q}^T\tilde{A}_k\tilde{Q})}^2\\
        \leq&{} \fnorm{\begin{bmatrix} \tilde{Q}^T(\tilde{A}_k - \lambda_{k1}I)\tilde{X}_1 &\dotsb & \tilde{Q}^T(\tilde{A}_k - \lambda_{km}I)\tilde{X}_m\end{bmatrix}}^2\\
        =&{} \fnorm{\begin{bmatrix} (\tilde{A}_k - \lambda_{k1}I)\tilde{X}_1 &\dotsb &(\tilde{A}_k - \lambda_{km}I)\tilde{X}_m\end{bmatrix}}^2.
    \end{split}
\end{equation}
By (\ref{eq:residue}), we have
\[
\begin{split}
    &\begin{bmatrix} (\tilde{A}_k - \lambda_{k1}I)\tilde{X}_1 &\dotsb &(\tilde{A}_k - \lambda_{km}I)\tilde{X}_m\end{bmatrix} \\
    =&{} \begin{bmatrix} (A_k - \lambda_{k1}I) (\lambda_1(\Vec{\mu})I - A(\Vec{\mu}))\pesudoinverse E(\Vec{\mu})Y_1 &\dotsb & (A_k - \lambda_{kn_m}I) (\lambda_m(\Vec{\mu})I - A(\Vec{\mu}))\pesudoinverse E(\Vec{\mu})Y_m\end{bmatrix} \\
    & + E_kY + \Ocal(\epsilon^2).
\end{split}
\]
Since $\eunorm{Y} \leq 1$, we have
\begin{equation}
\begin{split}
    &\fnorm{\begin{bmatrix} (\tilde{A}_k - \lambda_{k1}I)\tilde{X}_1 &\dotsb &(\tilde{A}_k - \lambda_{km}I)\tilde{X}_m\end{bmatrix}}  \\
    \leq&{} \fnorm{\begin{bmatrix} (A_k - \lambda_{k1}I) (\lambda_1(\Vec{\mu})I - A(\Vec{\mu}))\pesudoinverse E(\Vec{\mu})Y_1 &\dotsb & (A_k - \lambda_{kn_m}I) (\lambda_m(\Vec{\mu})I - A(\Vec{\mu}))\pesudoinverse E(\Vec{\mu})Y_m\end{bmatrix}}\\
    &+ \fnorm{E_k} +  \Ocal(\epsilon^2).
\end{split}
\end{equation}
Next, let 
\[C_{max}(\Vec{\mu}) = \max_{i \in \{1,\dots,m\}, k \in \{1,\dots,d\}}\{\eunorm{ (A_k - \lambda_{kn_i}I) (\lambda_{i}(\Vec{\mu})I - A(\Vec{\mu}))\pesudoinverse }\}.\]
Then, 
\begin{equation}
\begin{split} 
&\fnorm{\begin{bmatrix} (A_k - \lambda_{k1}I) (\lambda_1(\Vec{\mu})I - A(\Vec{\mu}))\pesudoinverse E(\Vec{\mu})Y_1 &\dotsb & (A_k - \lambda_{kn_m}I) (\lambda_m(\Vec{\mu})I - A(\Vec{\mu}))\pesudoinverse E(\Vec{\mu})Y_m\end{bmatrix}}^2\\
    =&{}\sum_{i=1}^{m}\fnorm{(A_k - \lambda_{kn_i}I) (\lambda_i(\Vec{\mu})I - A(\Vec{\mu}))\pesudoinverse E(\Vec{\mu})Y_i}^2\\
    \leq&{}\sum_{i=1}^{m}\eunorm{(A_k - \lambda_{kn_i}I) (\lambda_i(\Vec{\mu})I - A(\Vec{\mu}))\pesudoinverse}^2 \fnorm{ E(\Vec{\mu})Y_i}^2\\
    \leq&{} C_{max}(\Vec{\mu})^2 \sum_{i=1}^{m}\fnorm{ E(\Vec{\mu})Y_i}^2\\
    =&{} C_{max}(\Vec{\mu})^2 \fnorm{\begin{bmatrix}
    E(\Vec{\mu})Y_1 & \dotsb & E(\Vec{\mu})Y_m
    \end{bmatrix}}^2\\
    =&{} C_{max}(\Vec{\mu})^2 \fnorm{E(\Vec{\mu})Y}^2\\
    \leq&{} C_{max}(\Vec{\mu})^2 \fnorm{E(\Vec{\mu})}^2.
\end{split}
\end{equation}
The last inequality again follows from $\eunorm{Y} \leq 1$. Thus, combining (\ref{eq:offdiag_error}) (\ref{eq:error_split}) and (\ref{eq:first_error_term}),
\begin{equation}
    \fnorm{\offdiag(\tilde{Q}^T\tilde{A}_k\tilde{Q})}^2 \leq  C_{max}(\Vec{\mu})^2 \fnorm{E(\Vec{\mu})}^2 + 2C_{max}(\Vec{\mu})\fnorm{E(\Vec{\mu})}\fnorm{E_k}  + \fnorm{E_ k}^2 + \Ocal(\epsilon^3).
\end{equation}
Then
\begin{equation}
\begin{split}
    &\sum_{k=1}^{d}\fnorm{\offdiag(\tilde{Q}^T \tilde{A}_k \tilde{Q})}^2\\
    \leq&{} dC_{max}(\Vec{\mu})^2\fnorm{E(\Vec{\mu})}^2 + \sum_{k=1}^{d}2C_{max}(\Vec{\mu})\fnorm{E(\Vec{\mu})}\fnorm{E_k} + \sum_{k=1}^{d}\fnorm{E_k}^2 + \Ocal(\epsilon^3)\\
    \leq&{} dC_{max}(\Vec{\mu})^2\fnorm{E(\Vec{\mu})}^2  + 2C_{max}(\Vec{\mu})\sqrt{d}\fnorm{E(\Vec{\mu})}\epsilon + \epsilon^2 + \Ocal(\epsilon^3)\\
    \leq&{} ( 1 + \sqrt{d}C_{max}(\Vec{\mu})\eunorm{\Vec{\mu}})^2\epsilon^2 + \Ocal(\epsilon^3).
\end{split}
\end{equation}
The last inequality follows from $\fnorm{E(\Vec{\mu})}^2 \leq \eunorm{\Vec{\mu}}^2 \epsilon^2$ by Cauchy-Schwarz Inequality. Furthermore, if we assume $C_{max}(\Vec{\mu})\eunorm{\Vec{\mu}} \leq (R-1)/\sqrt{d}$, we have
\begin{equation}
 \sum_{k=1}^{d}\fnorm{\offdiag(\tilde{Q}^T \tilde{A}_k \tilde{Q})}^2\leq R^2\epsilon^2 + \Ocal(\epsilon^3).
 \end{equation}
Therefore, we would like to consider the random variable
\[X = \max_{i \in \{1,\dots,m\}, k \in \{1,\dots,d\}}\{\eunorm{ (A_k - \lambda_{kn_i}I)
(\lambda_{i}(\Vec{\mu})I - A(\Vec{\mu}))\pesudoinverse }\eunorm{\Vec{\mu}}\}.\]
We want the event $X < (R-1)/\sqrt{d}$ to happen. Hence, we consider the failure probability
\begin{equation}
    \begin{split}
            Pr\big( \exists i \in \{1,\dots,m\}, \exists k \in \{1,\dots,d\}, \eunorm{ (A_k - \lambda_{kn_i}I) (\lambda_i(\Vec{\mu})I - A(\Vec{\mu}))\pesudoinverse}\eunorm{\Vec{\mu}}  \geq \frac{R-1}{\sqrt{d}}\big).
    \end{split}
\end{equation}
Without loss of generality, we look at the matrix $(A_k - \lambda_{k1}I) (\lambda_1(\Vec{\mu})I - A(\Vec{\mu}))\pesudoinverse$ corresponding to the first ``group" of eigenvalues. Denote its $i$-th eigenvalues by $\alpha_{ki}$, we have
\[\alpha_{ki} = 
    \begin{cases}
    0, &  \lambda_{ki} = \lambda_{k1}, \\
    -(\lambda_{ki}- \lambda_{k1}) / \inner{\Vec{\Lambda }_i -\Vec{\Lambda}_1}{\Vec{\mu}}=-1 / \inner{\frac{\Vec{\Lambda}_i -\Vec{\Lambda}_1}{(\lambda_{ki}- \lambda_{k1})}}{\Vec{\mu}}, & \lambda_{ki} \neq \lambda_{k1}.
    \end{cases}
\]
Notice that for each $i$, since $\lambda_{ki} - \lambda_{k1}$ is not random, there exists a fixed $k_{max}(i)$ such that $\abs{\alpha_{k_{max}(i)i}}$ is the maximum among $\{\abs{\alpha_{ki}},i \in {1,\dots,n}\}$. Thus,
\begin{equation}
\begin{split}
    &Pr\big(\exists k \in \{1,\dots,d\}, \eunorm{ (A_k - \lambda_{kn_1}I) (\lambda_1(\Vec{\mu})I - A(\Vec{\mu}))\pesudoinverse}\eunorm{\Vec{\mu}}  \geq \frac{R-1}{\sqrt{d}}\big)\\
    =&{}Pr\big(\exists i \in [n], \abs{\alpha_{k_{max}(i)i}}\eunorm{\Vec{\mu}} \geq \frac{R-1}{\sqrt{d}}\big).
\end{split}
\end{equation}
If $\alpha_{ki} \neq 0$, we have for any $i \in \{1,\dots,n\}$,
\[ -\frac{1}{\alpha_{ki}} = \inner{\frac{\Vec{\Lambda}_i -\Vec{\Lambda}_1}{\lambda_{ki}- \lambda_{k1}}}{\Vec{\mu}}. \]
Then consider $1 / (\abs{\alpha_{ki}}\eunorm{\Vec{\mu}})$,
\[\frac{1}{\abs{\alpha_{ki}}\eunorm{\Vec{\mu}}} = \abs{\inner{\frac{\Vec{\Lambda}_i -\Vec{\Lambda}_1}{\lambda_{ki}- \lambda_{k1}}}{\frac{\Vec{\mu}}{\eunorm{\Vec{\mu}}}}}.\]
It is a well-known fact that normalized Gaussian vector $\Vec{\mu}/\eunorm{\Vec{\mu}}$ follows a uniform distribution over the unit sphere. And notice that 
\begin{equation}
    \eunorm{\frac{\Vec{\Lambda}_i -\Vec{\Lambda}_1}{\lambda_{ki}- \lambda_{k1}}} \geq 1
\end{equation} for $i$ such that $\lambda_{ki} \neq \lambda_{k1}$. Therefore,
\begin{equation}
\begin{split}
   Pr\big(\abs{\alpha_{ki}}\eunorm{\Vec{\mu}} \geq \frac{R-1}{\sqrt{d}}\big) &= Pr\big(\abs{\frac{1}{\alpha_{ki}\eunorm{\Vec{\mu}}}} \leq \frac{\sqrt{d}}{R-1}\big)\\
    &= Pr\big( \abs{\inner{\frac{\Vec{\Lambda}_i -\Vec{\Lambda}_1}{(\lambda_{ki}- \lambda_{k1})}}{\frac{\Vec{\mu}}{\eunorm{\Vec{\mu}}}}} \leq \frac{\sqrt{d}}{R-1}\big)\\
    &= Pr\big( \abs{\inner{\frac{\Vec{\Lambda}_i -\Vec{\Lambda}_1}{\eunorm{\Vec{\Lambda}_i - \Vec{\Lambda}_1}}}{\frac{\Vec{\mu}}{\eunorm{\Vec{\mu}}}}} \leq \frac{\sqrt{d}}{(R-1)\eunorm{\frac{\Vec{\Lambda}_i -\Vec{\Lambda}_1}{\lambda_{ki}- \lambda_{k1}}}}\big)\\
    &\leq Pr\big( \abs{\inner{\frac{\Vec{\Lambda}_i -\Vec{\Lambda}_1}{\eunorm{\Vec{\Lambda}_i - \Vec{\Lambda}_1}}}{\frac{\Vec{\mu}}{\eunorm{\Vec{\mu}}}}} \leq \frac{\sqrt{d}}{R-1}\big) \\
    &\leq \sqrt{\frac{2}{\pi}}\frac{d}{R-1}.
\end{split}
\end{equation}
The second last inequality follows from (\ref{eq:norm_bigger_than_one}), and the last inequality stems from   Lemma \ref{Probability Bound}. From the derivation we see that to bound each \[Pr(\abs{\alpha_{k_{max}(i)i}}\eunorm{\Vec{\mu}} \geq (R - 1)/\sqrt{d}),\]
we need to bound the inner product between $\Vec{\mu}/\eunorm{\Vec{\mu}}$ and $(\Vec{\Lambda}_i - \Vec{\Lambda}_1)/\eunorm{\Vec{\Lambda}_i - \Vec{\Lambda}_1}$ (for each event we need to bound along the direction $\Vec{\Lambda}_i - \Vec{\Lambda}_1$). But we have overall at most $\binom{m}{2} = m(m-1)/2$ different directions to consider for \[\Vec{\Lambda}_{n_i} - \Vec{\Lambda}_{n_j}, i,j \in \{1,\dots,m\} \wedge i \neq j.\] Thus, by applying a union bound with (\ref{eq:probability_for_one_eigenvalue}) to (\ref{eq:failure_event_2}) we have
\begin{equation}
    Pr(X \geq \frac{R-1}{\sqrt{d}})) \leq \frac{dm(m-1)}{\sqrt{2\pi}(R-1)} .
\end{equation}
Combining (\ref{eq:finalerror}) and (\ref{eq:failure_probability}), we get
\[ Pr\big( \sum_{k=1}^{d}\fnorm{\offdiag(\tilde{Q}^T \tilde{A}_k \tilde{Q})}^2\leq R^2\epsilon^2 + \Ocal(\epsilon^3)\big) \geq 1 -  \frac{dm(m-1)}{\sqrt{2\pi}(R-1)}.\]

\end{proof}
